# Supplementary material for: Modeling Insights from COVID-19 Incidence Data: Part II -- Why are compartment models so accurate?
Source: arXiv:2012.13424 ancillary file (2022-11-14)
Supplement: Supplementary file 1 [file Supplementary_Materials.pdf]

# Supplementary Materials

Ryan Wilkinson

January 11, 2021

The present Supplementary Materials document is meant to supplement the paper “Homogeneous Interpretable Approximations to Heterogeneous SIR Models” by Ryan Wilkinson and Marcus Roper. Figure references included herein refer to figures in the paper.

## 1 The Clustering Algorithm

### 1.1 The Distance Metric for Comparing State Case Curves

To cluster state curves, we must define distances between curves. Once this is done, existing clustering algorithms can be used to cluster curves. The formalism describing the distance metric used in this paper follows: Suppose we have time series  $\mathbf{X}$  and  $\mathbf{Y}$  for two different states, each with time series case data taken on the same even time interval (i.e. daily). Let  $X(i)$  be  $\mathbf{X}$ ’s data for the  $i$ th time point ( $\mathbf{X}$  and  $\mathbf{Y}$  need not have data defined on exactly the same set of days). For given shifts  $T$  and  $S$ , define the following function:

$$f(\mathbf{X}, \mathbf{Y}, T, S, \sigma) = \sqrt{\frac{1}{\text{length}(\mathbf{X})} \sum_{i=1}^{\text{length}(\mathbf{X})} \exp\left(\frac{(i - \text{length}(\mathbf{X}))^2}{2\sigma^2}\right)^2 (\log(X(i)) - (\log(Y(i - T)) + S))^2} \quad (\text{S1})$$

where  $T$  is an integer such that there are at least  $\min\{\text{length}(\mathbf{X}), \text{length}(\mathbf{Y})\}/4$  values of  $i$  such that  $\mathbf{X}(i)$  and  $\mathbf{Y}(i - T)$  are simultaneously defined.  $f$  measures the root mean squared distance between  $\log(\mathbf{X})$  and  $\log(\mathbf{Y})$  after  $\mathbf{Y}$  has been shifted to the right by  $T$  time points and has been scaled by a factor of  $S$ . This reflects an effort to compare cumulative case data in regions with different population sizes and epidemic start times. With  $f$  defined in Eq. S1, we define our distance metric  $d$ :

$$d(\mathbf{X}, \mathbf{Y}, \sigma) = \min \left\{ \min_{T \in \mathbb{Z}, S \in \mathbb{R}} f(\mathbf{X}, \mathbf{Y}, T, S, \sigma), \min_{T \in \mathbb{Z}, S \in \mathbb{R}} f(\mathbf{Y}, \mathbf{X}, T, S, \sigma) \right\} \quad (\text{S2})$$

Mathematically speaking, this is only formally a distance metric when “ $\mathbf{X} = \mathbf{Y}$ ” is defined to mean that there exists a shift and a scaling after which  $X(i) = Y(i)$  for at least  $\min\{\text{length}(\mathbf{X}), \text{length}(\mathbf{Y})\}/4$  consecutive time points. A more interpretable definition of  $d$  may be written as “the mean square distance of the log of the curves when one is allowed to shift curves left, right, up, and down until they fit the best.”

## 1.2 Constructing the Distance Heatmap and Clustering from Case Data

The US state data from [1] contains data from each of the 50 US states as well as data on the District of Columbia and Puerto Rico, leaving 52 cumulative case curves. We truncated data after May 20th to avoid considering pandemic resurgence dynamics which occurred in many of these regions in an effort to study initial SIR dynamics in each of the regions. We also truncated data in which there were fewer than 10 cases, including the beginning of epidemic data for some of the 52 states and territories, since these data are strongly affected by stochastic effects, and literal resemble the eventual spread of the disease. Once the data were truncated, we constructed a  $52 \times 52$  distance matrix from the metric  $d$  defined in Eq. S2 and choosing the value of 30 for  $\sigma$ . The heatmap was constructed directly from this matrix using the `imagesc` function in MATLAB. Hierarchical clustering was performed using the WPGMA algorithm [5] to separate the case data into 7 clusters. The number 7 was chosen in an ad hoc method by manual examination of the size and similarity of the clusters.

## 1.3 Visualization of the Case Curves after Shifting

To visualize clusters with  $d$ , the first region in the cluster was chosen as the reference curve, and the optimal shifts  $T$  and  $S$  were computed using  $d$  for each state. A plot was then formed showing each region's curve in the cluster in reference to the first curve after the optimal shifts had been performed. The solid black line in Fig. 1 was generated after fitting an SIR curve to the data using the method described in section 2 after adjusting the weight vector in the objective function for best visual results. Plots not included in Fig. 1 are shown in Fig. S1.

# 2 Fitting an SIR Curve to Case Data

There are many statistical methods to estimate parameters from data ([3, 4, 2], to name just a few). These often rely on assuming underlying distributions for errors in both the assumed model and the data. To reflect a complete ignorance of error distributions for the model and a lack of confidence in the data given, we opted for a simple approach. We derived the model parameters which produced the curve that fit the data well in a least-squares sense only. This objective is coincidentally equivalent to assuming Gaussian, time-independent error for the data, but was chosen mainly because minimizing least-squares error is a classical way of producing fits which “look” the best.

## 2.1 The Parameter Estimation Method

We have a model  $Y(t, \theta)$ , where  $t$  is a continuous variable and  $\theta$  is a vector of parameters, and a set of time points  $\{t_i\}$ ,  $i = 1, 2, \dots, n$ , upon which data  $X(t_i)$  are defined. Assume  $Y$  and  $X$  are vectors that are the same size. Fitting our model to the data means minimizing

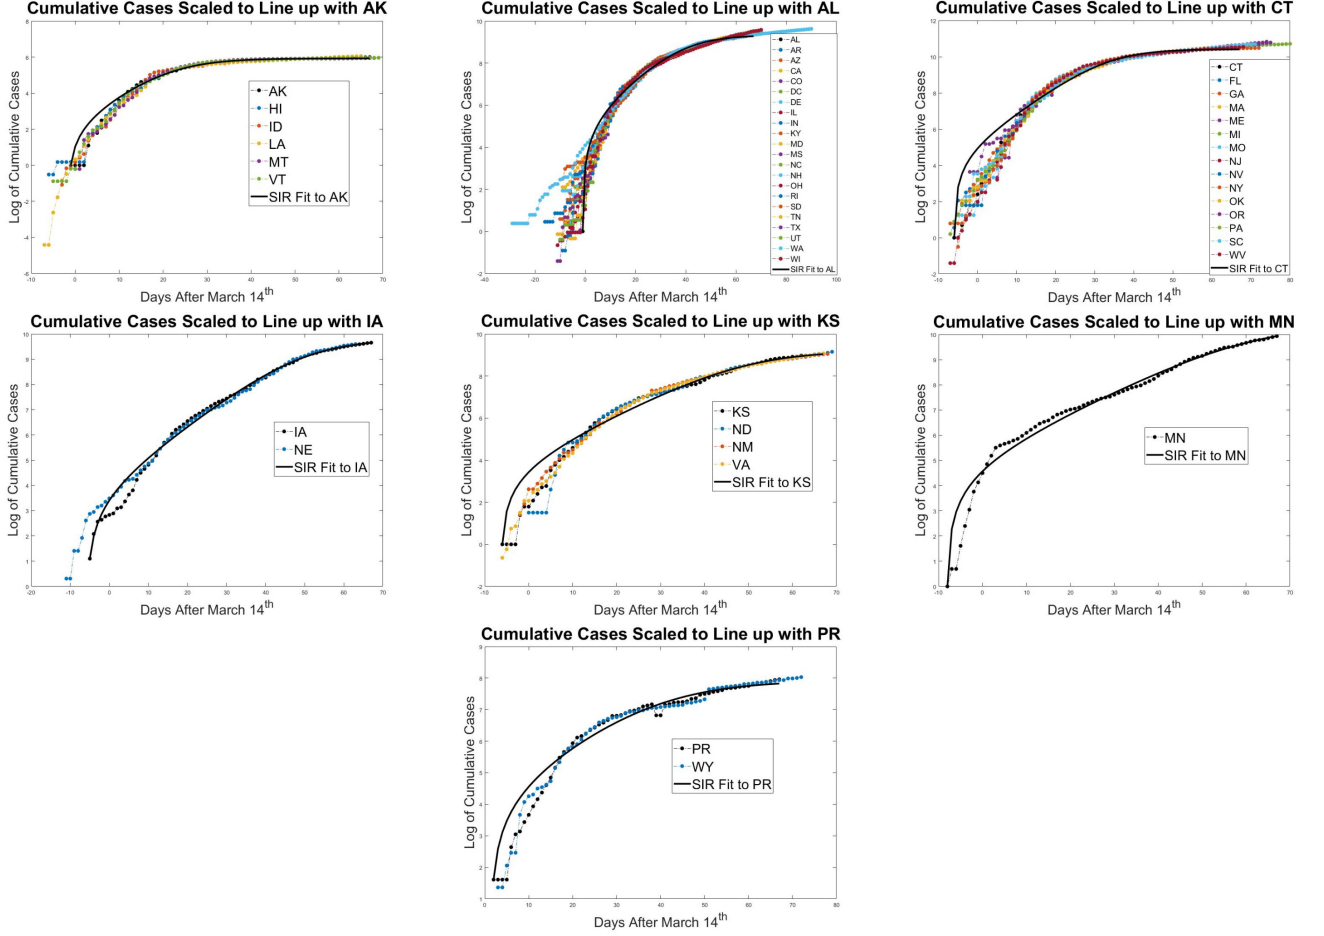

Figure S1: Shown are the computed clusters grouped together by the methods described above. The least-fitting cluster (in the authors' opinion) lining up with CT still fits reasonably well when the fit at later stages is considered, especially when one keeps in mind that case data is highly unreliable and sensitive to stochastic effects at the beginning of the pandemic.

the following objective function

$$E(\theta) = \sum_{i=1}^n w_i ||Y(t_i, \theta) - X(t_i)||^2 \quad (\text{S3})$$

for some set of weights  $w_i$ , whence the best-fitting parameter vector  $\hat{\theta}$  may be written as

$$\hat{\theta} = \arg \min_{\theta} E(\theta) \quad (\text{S4})$$

In this case, the model we desired to fit was the simple SIR model:

$$\begin{aligned}\frac{dS}{dt} &= -\beta SI/N_{tot} \\ \frac{dI}{dt} &= \beta SI/N_{tot} - \gamma I \\ \frac{dR}{dt} &= \gamma I\end{aligned}\tag{S5}$$

Since data was given in terms of cumulative cases, we have  $Y(t, \theta) = I(t) + R(t)$ , i.e. the number of people who are currently infected plus those that have been infected. In this case  $\theta = (\beta, \gamma, N_{tot}, S(0), I(0))$ . The model is differentiable with respect to  $\theta$ , so the minimum parameter vector may be found using gradient descent. Since the problem is non-convex, we optimized using many different initial guesses for  $\theta$  in an effort to coax out the global minimum from many different local minima. In an effort to keep  $\beta$  realistic, we also included constrained  $\gamma$  to be between 0 and 1, since  $\gamma$  (the disease removal rate) for COVID-19 can reasonably be assumed to be in that range, and almost certainly much smaller than 1. For best visual results such as those in the clustering analysis, we let  $w_i = t_i^p$  and adjusted  $p$  until the fit was to visual satisfaction.

## 2.2 Finding the Fitted $\beta$ for Simulated Data

For simulated data,  $N_{tot}$  was known and was included as a hyperparameter to the model, and so only  $\theta = \beta$  was considered. In order to better reflect fitting that happens on real data, the continuous simulated data was sampled at intervals one day apart, and the parameters used to generate the simulated data were chosen so that the timescale of the model was approximately one day for the COVID-19 pandemic. The weights  $w_i$  were set to 1 to fit the case data equally over the entire progression of the epidemic.

## 2.3 Two-Phase SIR Model Fitting

In an effort to fit state data when an SIR model with a single susceptibility parameter did poorly in fitting and to demonstrate applicability to later stages of the pandemic, we allowed the SIR model's susceptibility parameter to have two constant phases. Specifically, we considered the model

$$\begin{aligned}\frac{dS}{dt} &= -(\beta_1 + (\beta_2 - \beta_1)H(t - t^*))SI/N_{tot} \\ \frac{dI}{dt} &= (\beta_1 + (\beta_2 - \beta_1)H(t - t^*))SI/N_{tot} - \gamma I \\ \frac{dR}{dt} &= \gamma I\end{aligned}\tag{S6}$$

where  $H(t)$  is the Heaviside step function, namely  $H(t) = 1$  for  $t > 0$  and 0 otherwise. Given nondifferentiability in the  $t^*$  parameter, a grid search was formed over many values of  $t^*$  and the minimal error solution was saved. This approach better captured the behavior

of the (admittedly unreliably-reported) initial pandemic data and allowed for better overall curve fit. The model fits the worst-conforming state cluster (top right of Figure S1) in the cluster analysis(Fig S2). With two phases we can fit the data up to July 22nd. Given the

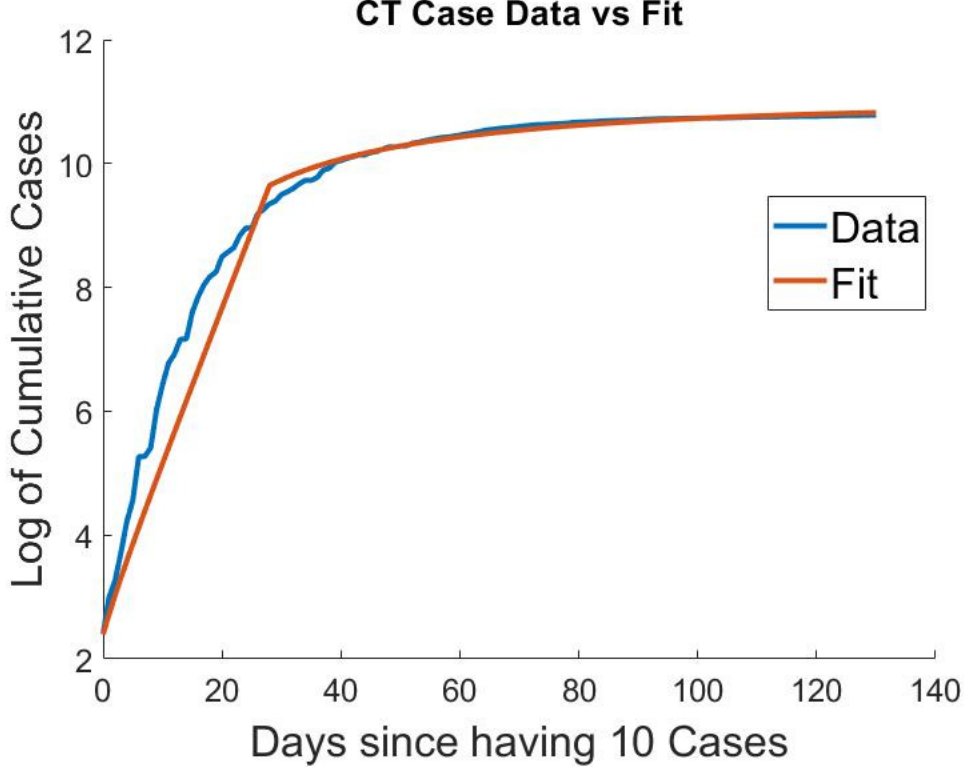

Figure S2: Demonstration of a two-phase SIR model fitting. The fit to CT is vastly improved by adding a susceptibility change degree of freedom to the minimization, representing a better overall fit to the entire top right cluster in Fig. S1.

interpretability argued in the paper, a single change to the basic susceptibility parameter corresponds with an abrupt change in interaction structure or interaction frequency (by changing the  $b$  parameter).

### 3 Deriving $\tilde{\beta}$ and its Interpretations

To determine the optimal value of  $\tilde{\beta}$  for approximating a heterogeneous population a simple SIR model, we find the  $\tilde{\beta}$  which results in the minimization of the off-SIR terms relative to the SIR term, i.e. minimizing the size of the function

$$F(\tilde{\beta}, t) \equiv \frac{\sum_{i=1}^K \sum_{j=1}^K \left( \frac{\beta_{ij}}{N_j} - \frac{\tilde{\beta}}{N_{tot}} \right) S_i I_j}{\frac{\tilde{\beta}}{N_{tot}} SI} \quad (S7)$$

For differentiability, we chose to minimize the  $L^2$  norm of this function over an arbitrary time interval  $(t_1, t_2)$ . Such a minimum occurs when  $\int_{t_1}^{t_2} \frac{\partial}{\partial \tilde{\beta}} (F(\tilde{\beta}, t)^2) dt = 0$ , or when:

$$\tilde{\beta} = N_{tot} \frac{\int_{t_1}^{t_2} \frac{\left( \sum_{i=1}^K \sum_{j=1}^K \frac{\beta_{ij}}{N_j} S_i I_j \right)^2}{(SI)^2} dt}{\int_{t_1}^{t_2} \frac{\sum_{i=1}^K \sum_{j=1}^K \frac{\beta_{ij}}{N_j} S_i I_j}{SI} dt} \quad (S8)$$

### 3.1 Asymptotic Results for $\tilde{\beta}$

We assume that  $\beta_{ij}$  is given by Eqn (4), reproduced here:

$$\beta_{ij} = \beta \left( \left( b \frac{N_j}{N_{tot}} + (1-b) \right) \delta_{ij} + b \frac{N_j}{N_{tot}} (1 - \delta_{ij}) A_{ij} \right) \quad (S9)$$

We make an additional asymptotic assumption to make sense of Eq. S8: namely that  $N_i = N + \varepsilon_i$ ,  $\varepsilon_i \ll N$ , where  $N := N_{tot}/K$  is the average subpopulation size. In the paper,  $N_i = N$ , so asymptotic results derived here are in fact exact for that regime. Under this assumption, the sum term in the multi-compartment model changes to:

$$\sum_{i=1}^K \sum_{j=1}^K \frac{\beta_{ij}}{N_j} S_i I_j = \frac{\beta}{N_{tot}} \left( (K - (K-1)b) \sum_{i=1}^K S_i I_i + b \sum_{i=1}^K \sum_{j=1}^K A_{ij} S_i I_j \right) + \mathcal{O}\left(\frac{\varepsilon_i}{N}\right)$$

After a lot of algebraic massaging, we reduce  $\tilde{\beta}$  to

$$\tilde{\beta} = \beta \frac{\int_{t_1}^{t_2} \left( \frac{K-(K-1)b}{K} \left( 1 + K \sum_{i=1}^K \frac{S_i}{S} \left( \frac{I_i}{I} - \frac{1}{K} \right) \right) + b \frac{\sum_{i=1}^K \sum_{j=1}^K A_{ij} S_i I_j}{SI} + \mathcal{O}\left(\frac{\varepsilon_i}{N}\right) \right)^2 dt}{\int_{t_1}^{t_2} \frac{K-(K-1)b}{K} \left( 1 + K \sum_{i=1}^K \frac{S_i}{S} \left( \frac{I_i}{I} - \frac{1}{K} \right) \right) + b \frac{\sum_{i=1}^K \sum_{j=1}^K A_{ij} S_i I_j}{SI} + \mathcal{O}\left(\frac{\varepsilon_i}{N}\right) dt}$$

When  $A_{ij}$  is the adjacency matrix for a complete graph, this expression is further simplified to

$$\begin{aligned} \tilde{\beta} &= \beta \frac{1 + \frac{1}{t_2-t_1} \int_{t_1}^{t_2} (1-b) \left[ K \sum_{i=1}^K \frac{S_i}{S} \left( \frac{I_i}{I} - \frac{1}{K} \right) \right] \left( 2 + (1-b) \left[ K \sum_{i=1}^K \frac{S_i}{S} \left( \frac{I_i}{I} - \frac{1}{K} \right) \right] \right) + \mathcal{O}\left(\frac{\varepsilon_i}{N}\right) dt}{1 + \frac{1}{t_2-t_1} \int_{t_1}^{t_2} (1-b) \left[ K \sum_{i=1}^K \frac{S_i}{S} \left( \frac{I_i}{I} - \frac{1}{K} \right) \right] + \mathcal{O}\left(\frac{\varepsilon_i}{N}\right) dt} \\ &= \beta \left( 1 + \frac{\frac{1}{t_2-t_1} \int_{t_1}^{t_2} (1-b) \left[ K \sum_{i=1}^K \frac{S_i}{S} \left( \frac{I_i}{I} - \frac{1}{K} \right) \right] \left( 1 + (1-b) \left[ K \sum_{i=1}^K \frac{S_i}{S} \left( \frac{I_i}{I} - \frac{1}{K} \right) \right] \right) + \mathcal{O}\left(\frac{\varepsilon_i}{N}\right) dt}{1 + \frac{1}{t_2-t_1} \int_{t_1}^{t_2} (1-b) \left[ K \sum_{i=1}^K \frac{S_i}{S} \left( \frac{I_i}{I} - \frac{1}{K} \right) \right] + \mathcal{O}\left(\frac{\varepsilon_i}{N}\right) dt} \right) \end{aligned} \quad (S10)$$

These unruly equations are surprisingly interpretable: graph structure matters more as mixing parameter  $b$  increases, and asymmetrical subpopulation dynamics matter more as mixing parameter  $b$  decreases. When  $A_{ij}$  is a complete adjacency matrix, we see that, as  $b$  approaches 1, we will always recover  $\tilde{\beta} = \beta$  exactly so long as subpopulations have the same size. The rate at which  $\tilde{\beta}$  approaches  $\beta$  is bundled up into the complicated fraction of integrals, but, surprisingly, the fraction in the last part of Eq. S10 seems always to be

negative for the initial conditions we tried as evidenced by Fig. 2. A heuristic for why this is true is due to the interpretation of the sum terms as a covariance. Specifically:

$$\sum_{i=1}^K \frac{S_i}{S} \left( \frac{I_i}{I} - \frac{1}{K} \right) = \sum_{i=1}^K \left( \frac{S_i}{S} - \frac{1}{K} \right) \left( \frac{I_i}{I} - \frac{1}{K} \right) = \text{Cov}\left(\frac{S_i}{S}, \frac{I_i}{I}\right)$$

This is in general negative, because high  $I_i$  is associated with a reduced susceptible population in a given subcompartment.

## References

- [1] *The covid tracking project*, <https://covidtracking.com/>. 1.2
- [2] Arnaud Doucet and Adam M Johansen, *A tutorial on particle filtering and smoothing: Fifteen years later*, Handbook of nonlinear filtering **12** (2009), no. 656-704, 3. 2
- [3] Rudolph Emil Kalman, *A new approach to linear filtering and prediction problems*, Transactions of the ASME–Journal of Basic Engineering **82** (1960), no. Series D, 35–45. 2
- [4] In Jae Myung, *Tutorial on maximum likelihood estimation*, Journal of Mathematical Psychology **47** (2003), no. 1, 90 – 100. 2
- [5] Robert R. Sokal and Charles D. Michener, *A statistical method for evaluating systematic relationships*, The University of Kansas Science Bulletin **38** (1958), 1409–1438. 1.2
